# Supplementary material for: A Systematic Procedure for Topological Path Identification with Raw Data Transformation in Electrical Distribution Networks
Source: arXiv:2409.09075 source file (2024-09-09)
Supplement: Supplementary file 1 [file appendices.tex]

\appendices
\section{Pseudo-algorithms}

\begin{algorithm}
\caption{Connect Underground Lines to Armoires algorithm}
\begin{algorithmic}[1]
    \REQUIRE Set of all elements: $E$
    \REQUIRE Maximum distance threshold: $D$
    % \ENSURE List of pairs $(n^*, m^*)$ representing feasible connections: $L$
    
    \STATE Initialize an empty list $L$
    
    \FOR{each element $e$ in $Subset(\mathcal{E}, underground)$}
        \STATE Initialize $t$ as \textit{None}
        \STATE Initialize $l$ as \textit{None}
        \STATE $n^* = Closest(e^1, Subset(\mathcal{E}, armoire))$
        \STATE $m^* = Closest(e^{|e|}, Subset(\mathcal{E}, armoire))$
    
        \IF{ $Dist(e^1, n^*) < D$ and $Dist(e^{|e|}, m^*) < D$ and $n^* \neq m^*$}
            \STATE Set $l$ as $(COOR(n^*), COOR(m^*))$
            \STATE Set $t$ as $underground$
            \STATE Set the type of $l$ as $t$
            \STATE Append the pair $l$ to the list $L$
        \ENDIF
    \ENDFOR
    \STATE Substitute $Subset(\mathcal{E}, underground)$ with $L$
    \RETURN $\mathcal{E}$
\end{algorithmic}
\end{algorithm}

\begin{algorithm}
\caption{Connect customers to main feeder algorithm}
\begin{algorithmic}[1]
    \REQUIRE Set of all elements: $E$
    % \ENSURE List of pairs $(n^*, m^*)$ representing feasible connections: $L$
    
    \STATE Initialize an empty list $L$
    
    \FOR{each element $e$ in $Subset(\mathcal{E}, customer)$}
        \STATE Initialize $t$ as \textit{None}
        \STATE Initialize $l$ as \textit{None}
        \STATE $n^* = Closest(e, Subset(\mathcal{E}, armoire))$
        \STATE $m^* = Closest(e, Subset(\mathcal{E}, pole))$
    
        \IF{ $Dist(e, n^*) < Dist(e, m^*)$}
            \STATE Set $l$ as $(Coor(e), Coor(n^*))$
            \STATE Set $t$ as $armoire$
        \ELSE
            \STATE Set $l$ as $(Coor(e), Coor(m^*))$
            \STATE Set $t$ as $pole$
        \ENDIF
        \STATE set the type of $l$ as $t$
        \STATE Append the pair $l$ to the list $L$
    \ENDFOR
    
    \STATE Add $L$ to $\mathcal{E}$
    \RETURN $\mathcal{E}$
\end{algorithmic}
\end{algorithm}

\begin{algorithm}
\caption{Find switches location algorithm}
\begin{algorithmic}[1]
    \REQUIRE Set of all elements: $E$
    % \ENSURE List of pairs $(n^*, m^*)$ representing feasible connections: $L$

    \STATE Initialise $\mathcal{S}$ as $None$
    \STATE $\mathcal{S} = HumanInspection()$
    
    \STATE Add $\mathcal{S}$ to $\mathcal{E}$
    \RETURN $\mathcal{E}$
\end{algorithmic}
\end{algorithm}

\begin{algorithm}
\caption{Generate graph algorithm}
\begin{algorithmic}[1]
    \REQUIRE Set of all elements: $\mathcal{E}$
    % \ENSURE List of pairs $(n^*, m^*)$ representing feasible connections: $L$

    \STATE TO BE DEFINED (not the focus of this work?)
    
    % \STATE add $\mathcal{E}'$ to $\mathcal{E}$
    \RETURN $\mathcal{G}$
\end{algorithmic}
\end{algorithm}

\begin{algorithm}
\caption{Iterative helper function paths}
\begin{algorithmic}[1]
    \REQUIRE Graph: $\mathcal{G}$
    \REQUIRE Customer element: $e$
    \REQUIRE Set of all elements: $\mathcal{E}$
    \REQUIRE Steps Counter: $k$
    \REQUIRE Set of all already visited elements: $V$
    
    \STATE Set $N$ as the maximum number of steps
    \STATE $e_{nexts}$ = FindConnectedElements($\mathcal{G}$, $e$)

    \FOR{each element $e_{next}$ in $e_{nexts}$}
        \IF{$Type(e_{next}) == transformer$}
            \RETURN $V$
        \ELSIF{$e_{next} \in V$ or $k > N$}
            \RETURN $NONE$
        \ELSE
            \STATE Add $e$ to $V$
            \STATE k = k + 1
            \STATE $Paths(\mathcal{G}, e_{next}, \mathcal{E}, k, V)$
        \ENDIF
    \ENDFOR
\end{algorithmic}
\end{algorithm}

\begin{algorithm}
\caption{Find compatible hypothetical paths}
\begin{algorithmic}[1]
    \REQUIRE Set of all elements: $\mathcal{E}$
    \REQUIRE Set of all information: $\mathcal{I}$
    \REQUIRE Set of all assumptions: $\mathcal{A}$
    
    \FOR{each element $e$ in $Subset(\mathcal{E}, customer)$}
        \STATE Initialise $h$ as $None$

        h = $Paths(\mathcal{G}, e, \mathcal{E}, 0, \{\})$
        \IF{h is not $None$}
            \STATE Add $h$ to $\hat{\mathcal{H}}^{(\mathcal{I},\mathcal{A})}$
        \ENDIF
    \ENDFOR

    \RETURN $\hat{\mathcal{H}}^{(\mathcal{I},\mathcal{A})}$
\end{algorithmic}
\end{algorithm}

\begin{algorithm}
\caption{Main algorithm}
\label{algo:meth}
\begin{algorithmic}[1]
    \REQUIRE set of elements $\mathcal{E}$
    \REQUIRE set of types $\mathcal{T}$
    \REQUIRE set of information $\mathcal{I}$
    \REQUIRE set of assumptions $\mathcal{A}$
    % \ENSURE The sum of the first $n$ positive integers
    % \STATE $sum \gets 0$
    \STATE $\mathcal{E} = ConnectUndergroundLines2Armoires(\mathcal{E})$
    \STATE $\mathcal{E} = ConnectCustomers2Feeder(\mathcal{E})$
    \STATE $\mathcal{E} = LocateSwitches()$
    \STATE $\mathcal{G} = GenerateGraph(\mathcal{E})$
    \STATE $\hat{\mathcal{H}}^{(\mathcal{I},\mathcal{A})} = 
    FindPaths(\mathcal{G},\mathcal{E},\mathcal{I},\mathcal{A})$
\end{algorithmic}
\end{algorithm}
